# Supplementary material for: Modulation of Point Defect Properties Near Surfaces in Metal Halide Perovskites
Source: arXiv:2407.02249 source file (2024-07-02)
Supplement: Supplementary file 1 [file suppinfo.pdf]

# Supporting Information: Modulation of Point Defect Properties Near Surfaces in Metal Halide Perovskites

Bilal Ahmad, Md Salman Rabbi Limon, and Zeeshan Ahmad*

*Department of Mechanical Engineering, Texas Tech University, Lubbock, Texas 79409, USA*

E-mail: zeeahmad@ttu.edu

## Method Details

The structures used for MAPI and $CsPbI_3$ in our study are orthorhombic. For the calculation of defect formation energies in the bulk, 2×2×2 supercell consisting of 80 atoms for $CsPbI_3$ and $\sqrt{2}\times\sqrt{2}\times1$ supercell consisting of 96 atoms for MAPI, were used. The value of $\Delta_{\text{corr}}$ for the vacancy and interstitial defects in different charge states for both MAPI and $CsPbI_3$ are shown in Table S1. For all the slabs (001), the vacuum region of length 10 Å on each side of slabs was used. We used atomic simulation environment[1] for generating supercells and surfaces. VESTA[2] was used for the visualization purpose.

# $\Delta_{corr}$ : For MAPI and $CsPbI_3$ supercells

Table S1: Value of $\Delta_{corr}$ for MAPI and $CsPbI_3$ supercells for both vacancy and interstitial defects in the bulk.

| **Defect** | $\mathbf{\Delta_{corr}}$ **(eV)** | **Defect** | $\mathbf{\Delta_{corr}}$ **(eV)** |
|---|---|---|---|
| MAPI $V_I^{\bullet}$ | -0.1170 | $CsPbI_3$ $V_I^{\bullet}$ | 0.02 |
| MAPI $V_I^{\prime}$ | 0.1776 | $CsPbI_3$ $V_i^{\prime}$ | 0.1895 |
| MAPI $I_i^{\bullet}$ | 0.1933 | $CsPbI_3$ $I_i^{\bullet}$ | 0.1849 |
| MAPI $I_i^{\prime}$ | -0.1508 | $CsPbI_3$ $I_i^{\prime}$ | -0.0708 |

# Lattice Parameters : For MAPI and $CsPbI_3$ unit cells

Table S2: Lattice Parameters for MAPI and $CsPbI_3$

| **Lattice Parameters** | **MAPI (Å)** | $\mathbf{CsPbI_3}$ **(Å)** |
|---|---|---|
| $a$ | 8.8362 | 8.8560 |
| $b$ | 8.5551 | 8.5760 |
| $c$ | 12.5804 | 12.4720 |

In Fig S3, we plot the out of plane and in-plane I-I distances near the defect as a function of the distance from the surface, for various defect locations in different layers of MAPI. For vacancy defects (panels a and b), the deviation of out of plane I-I distances is relatively larger than the interstitial defects. While for in-plane I-I distances, the deviation is smaller than the interstitial defects. As we can observe that for interstitial defects [(c) and (d)], there were significant deviations in the in-plane I-I distances as well.

In Figure S4, the plot show the out-of-plane and in-plane I-I distances near defects as a function of their distance from the surface for different defect positions in various $CsPbI_3$ layers. For vacancy defects (panels a and b), the deviation of in-plane I-I distances is very less as compared to interstitial defects. On the other hand, in case of interstitial defects (panels c and d), the in-plane I-I distances deviate over a significant range.

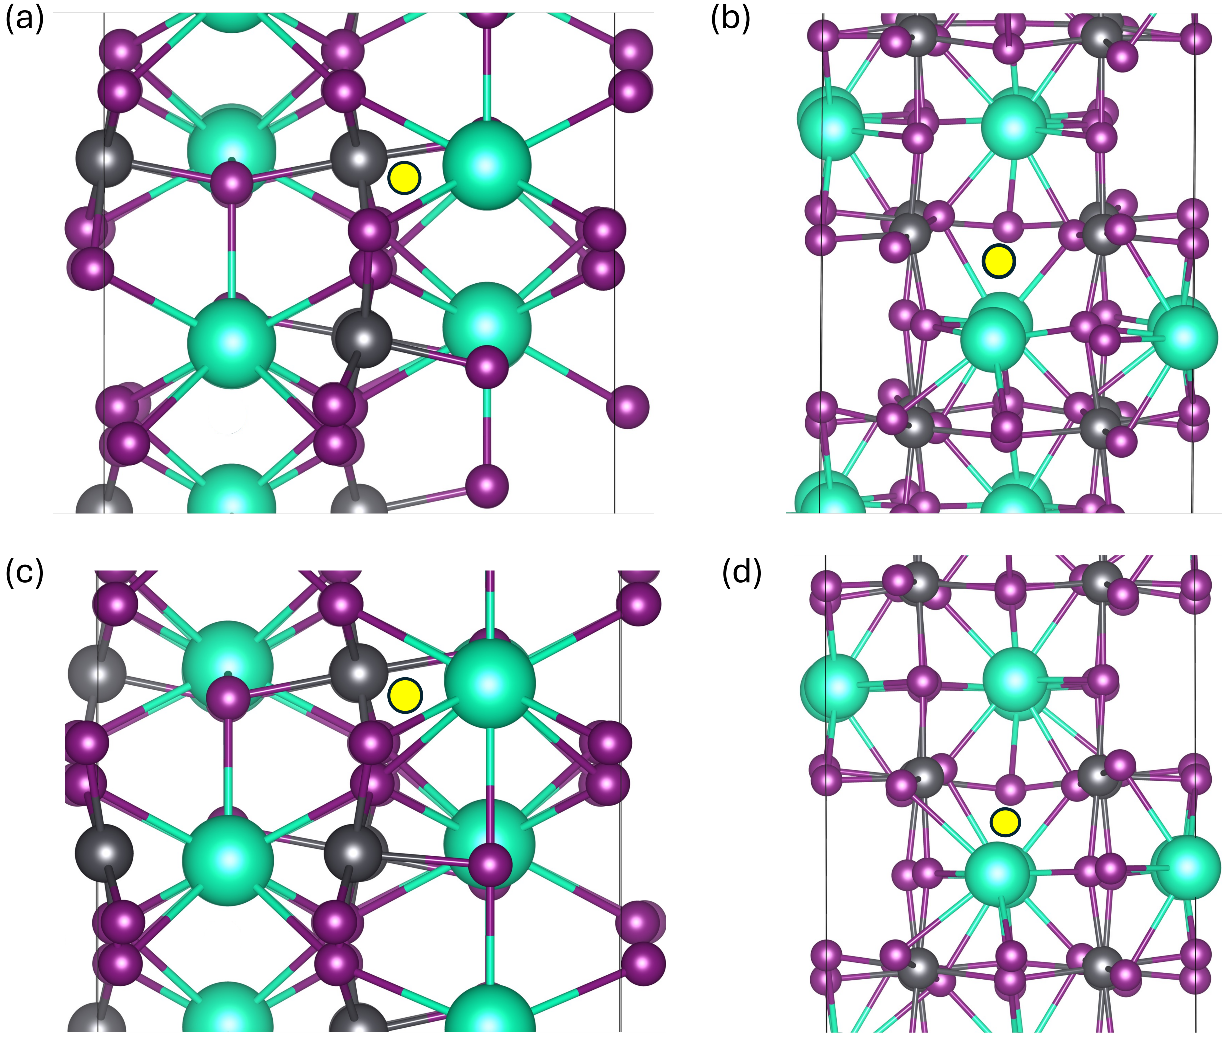


Figure S1: Depiction of iodine vacancies in $CsPbI_3$. Iodine vacancies are represented by yellow circles. This figure shows (a) $V_I^{\bullet}$ in bulk, (b) $V_I^{\bullet}$ at surface, (c) $V_i'$ in bulk, and (d) $V_i'$ at surface.

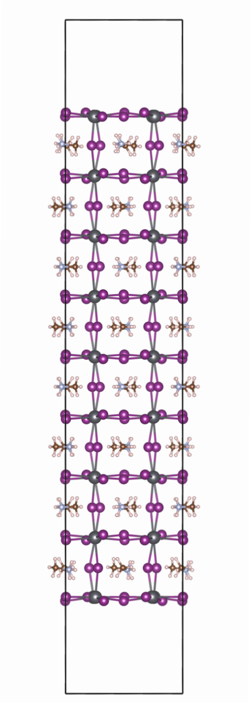

Figure S2: Depiction of 17-layer MAPI slab. It consists of alternating layers of $PbI_2$ and MAI. Vacuum of 10 Å is considered on both sides of the slab.

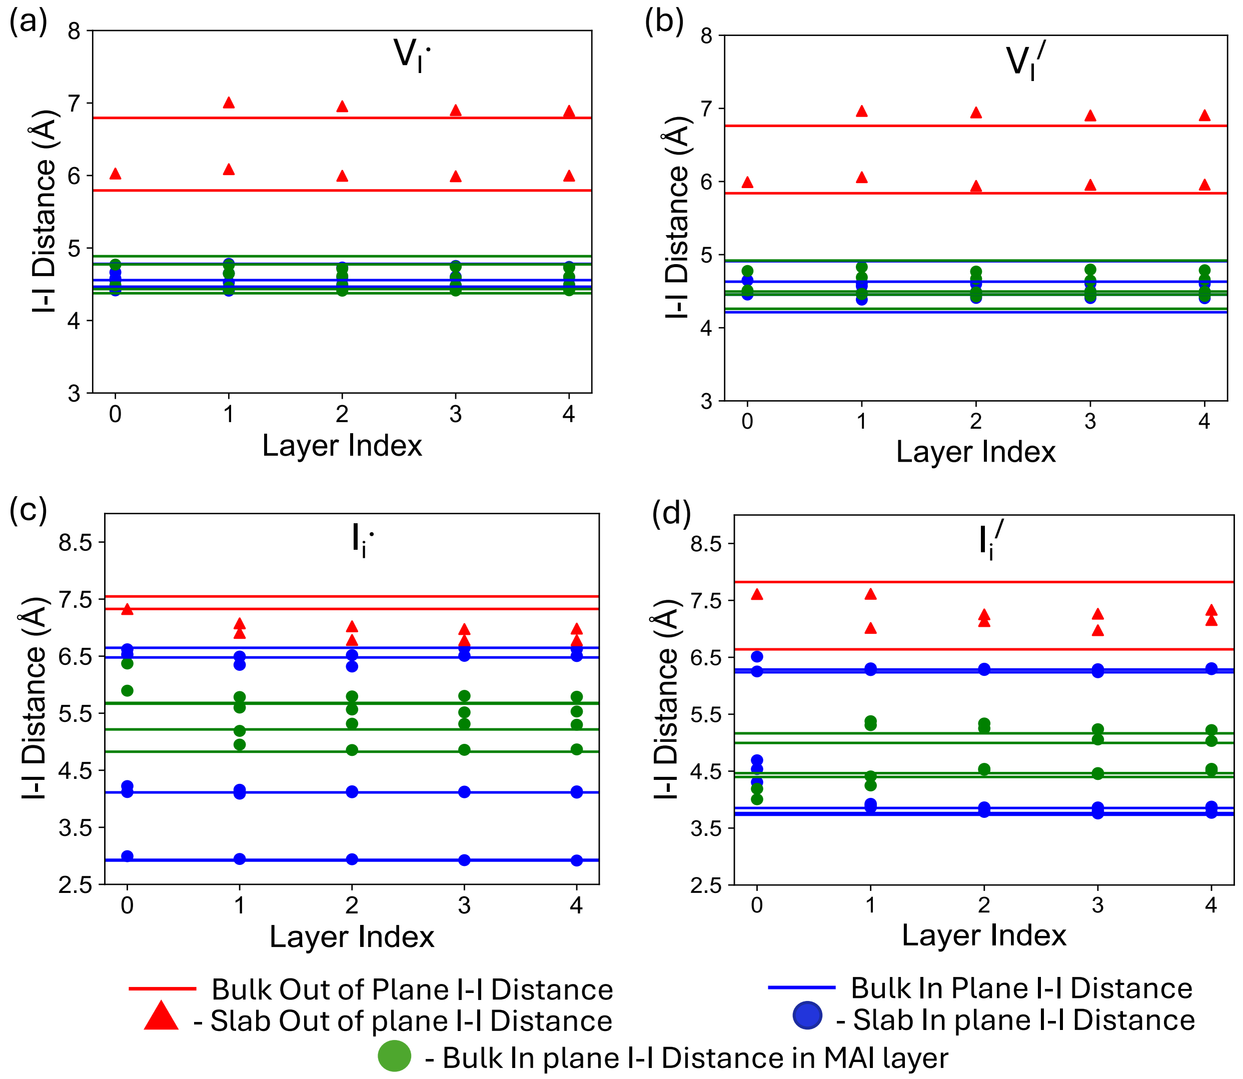


Figure S3: In plane and out of plane I-I distances in MAPI plotted against the layer index from the surface for (a) $V_I^{\bullet}$, (b) $V_I^{\prime}$, (c) $I_i^{\bullet}$, and (d) $I_i^{\prime}$, respectively.

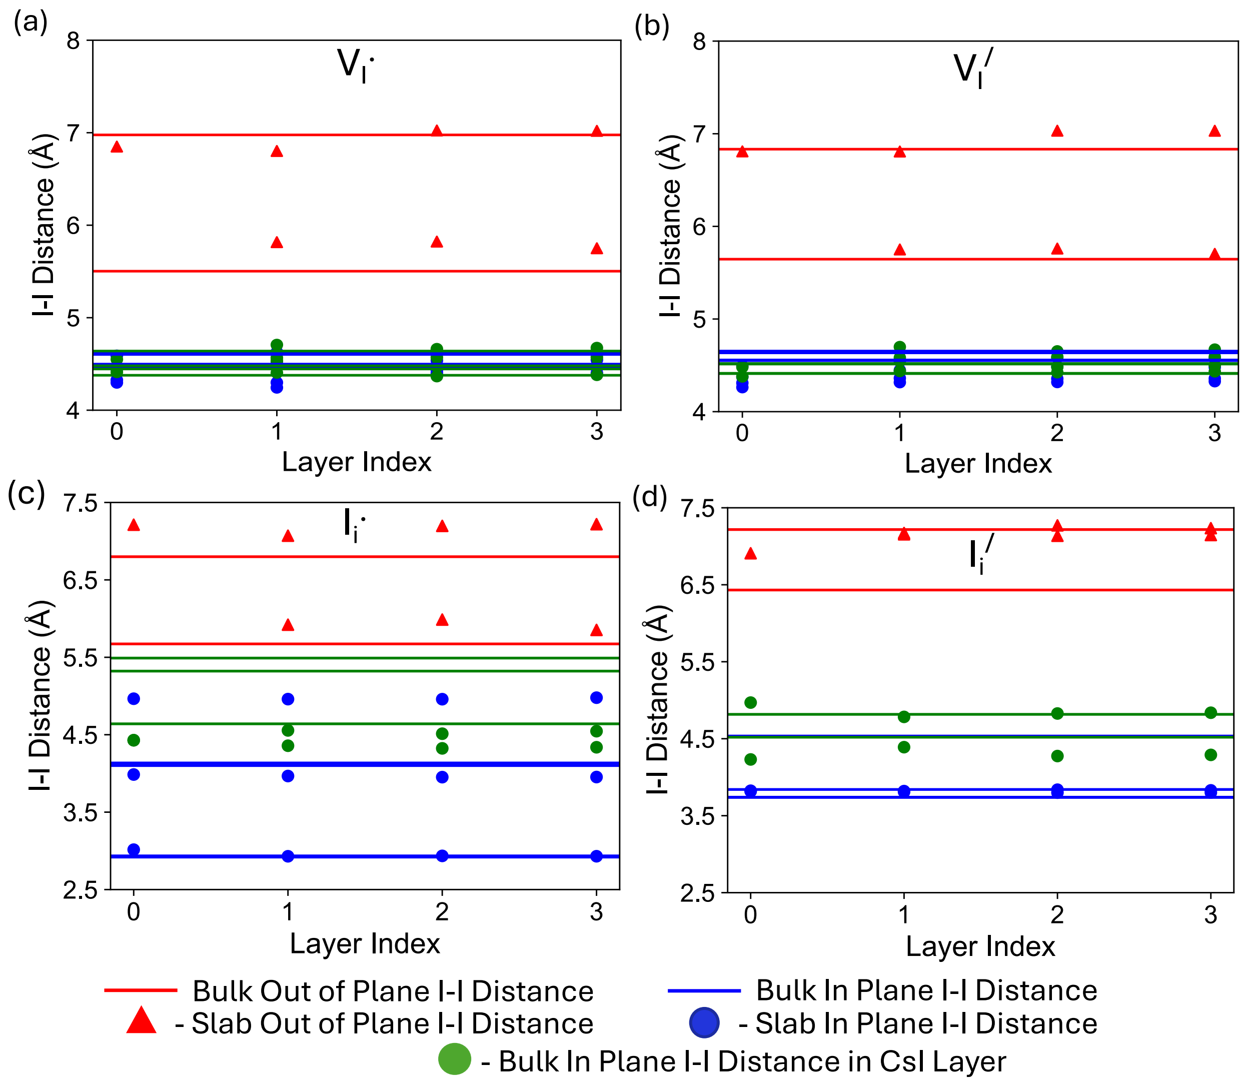


Figure S4: In plane and out of plane I-I distances in $CsPbI_3$ plotted against the layer index showing the comparison of I-I distances in the bulk and on the surface layers for (a) $V_I^{\bullet}$, (b) $V_I^{\prime}$, (c) $I_i^{\bullet}$, and (d) $I_i^{\prime}$, respectively.

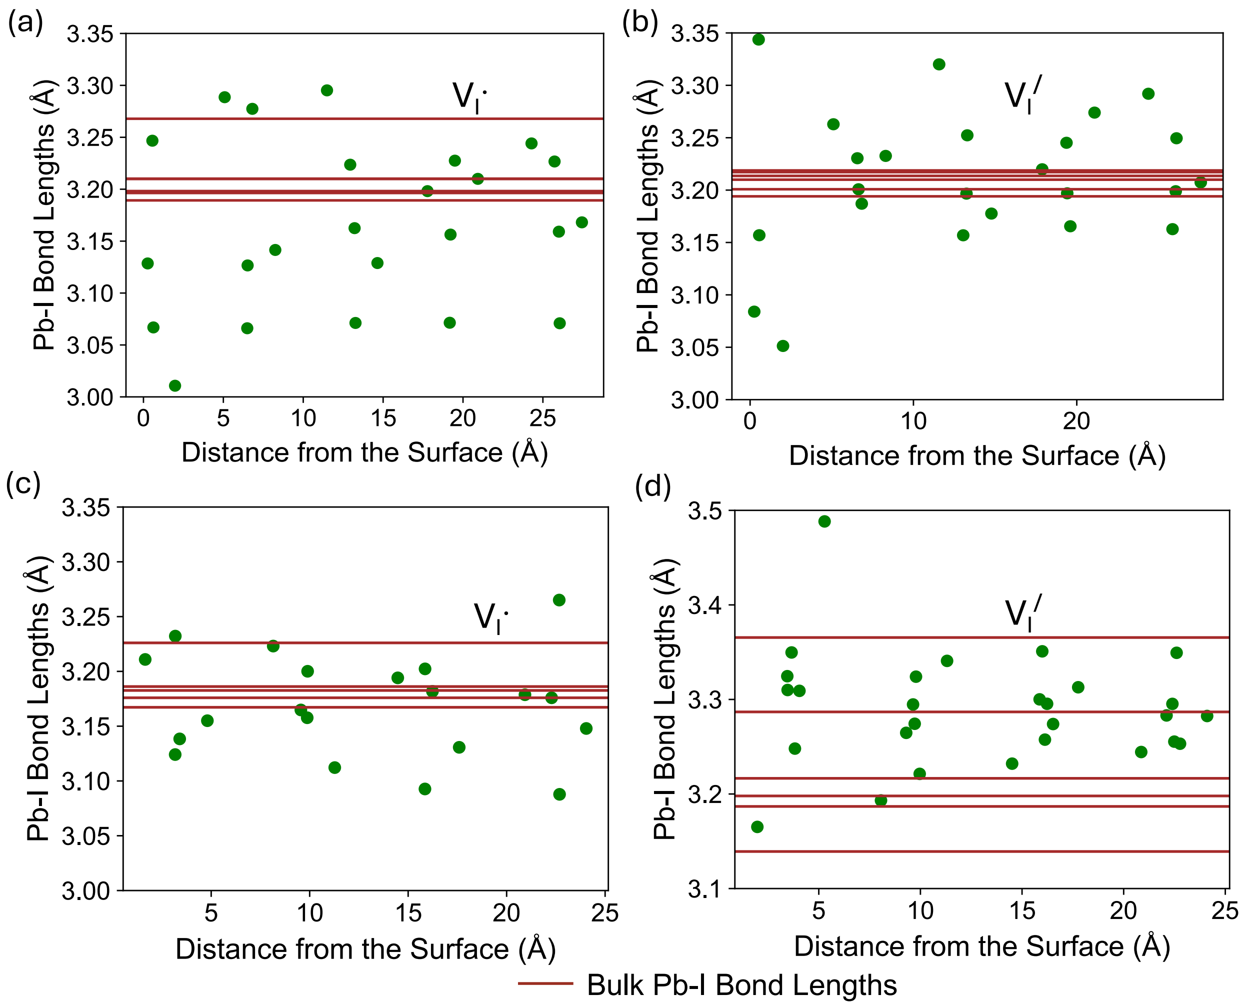


Figure S5: Pb-I bond lengths for vacancy defects in MAPI and $CsPbI_3$ plotted against the distance of the defects showing variation for (a) $V_I^{\bullet}$ in MAPI, (b) $V_I^{\prime}$ in MAPI, (c) $V_I^{\bullet}$ in $CsPbI_3$, and (d) $V_I^{\prime}$ in $CsPbI_3$, respectively.

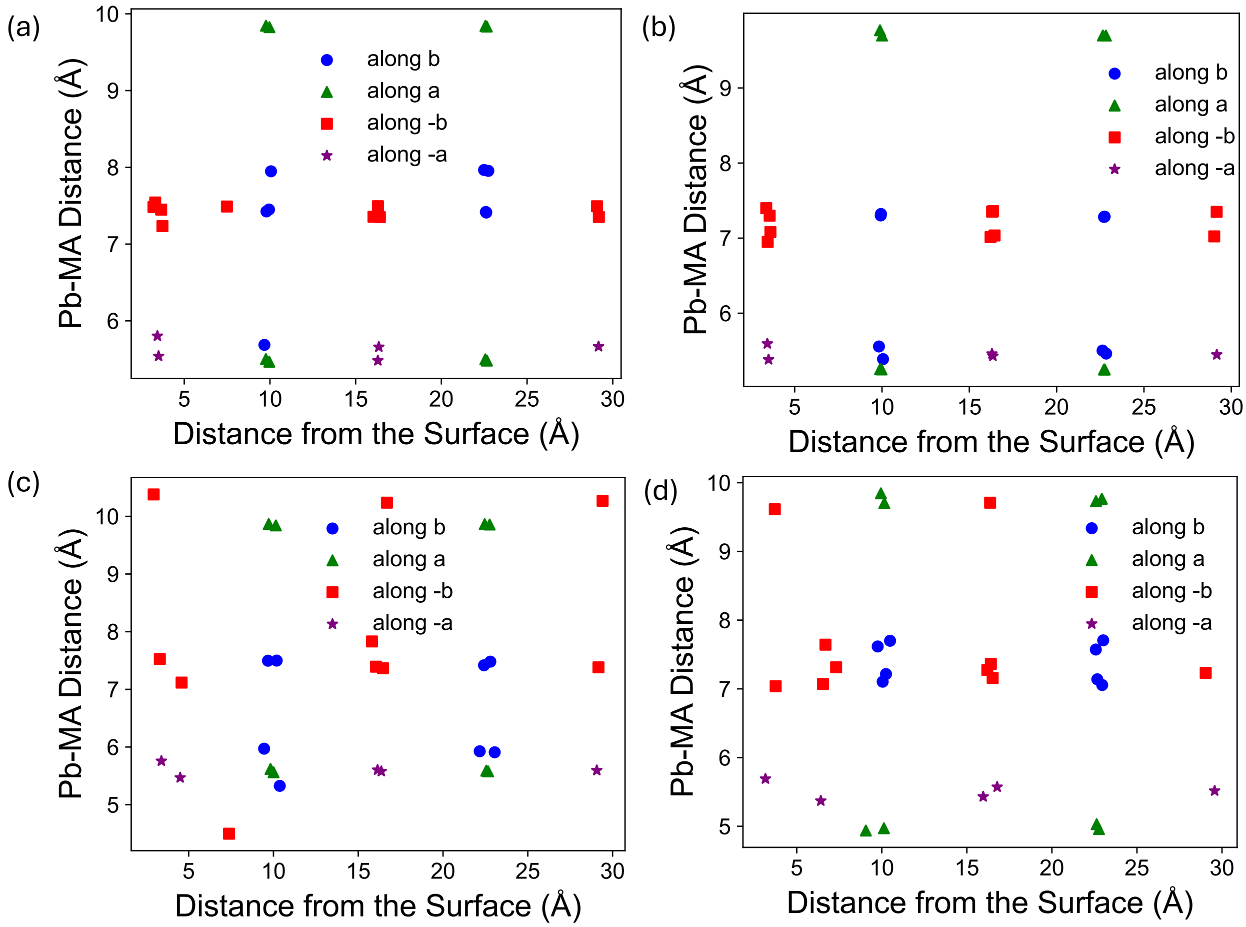


Figure S6: Pb-MA distances plotted against the location of defects based on different orientations of MA group in MAPI. This figure represents the variation of Pb-MA distance for (a) $V_I^{\bullet}$, (b) $V_I^{\prime}$, (c) $I_i^{\bullet}$ and (d) $I_i^{\prime}$. MA group with the direction vector along C to N in x-direction is shows by green triangles and in y direction is shown by blue circles. Similarly, the prientation of MA group along C to N in negative x-direction is shown by purple stars and in negative y direction by red squares.

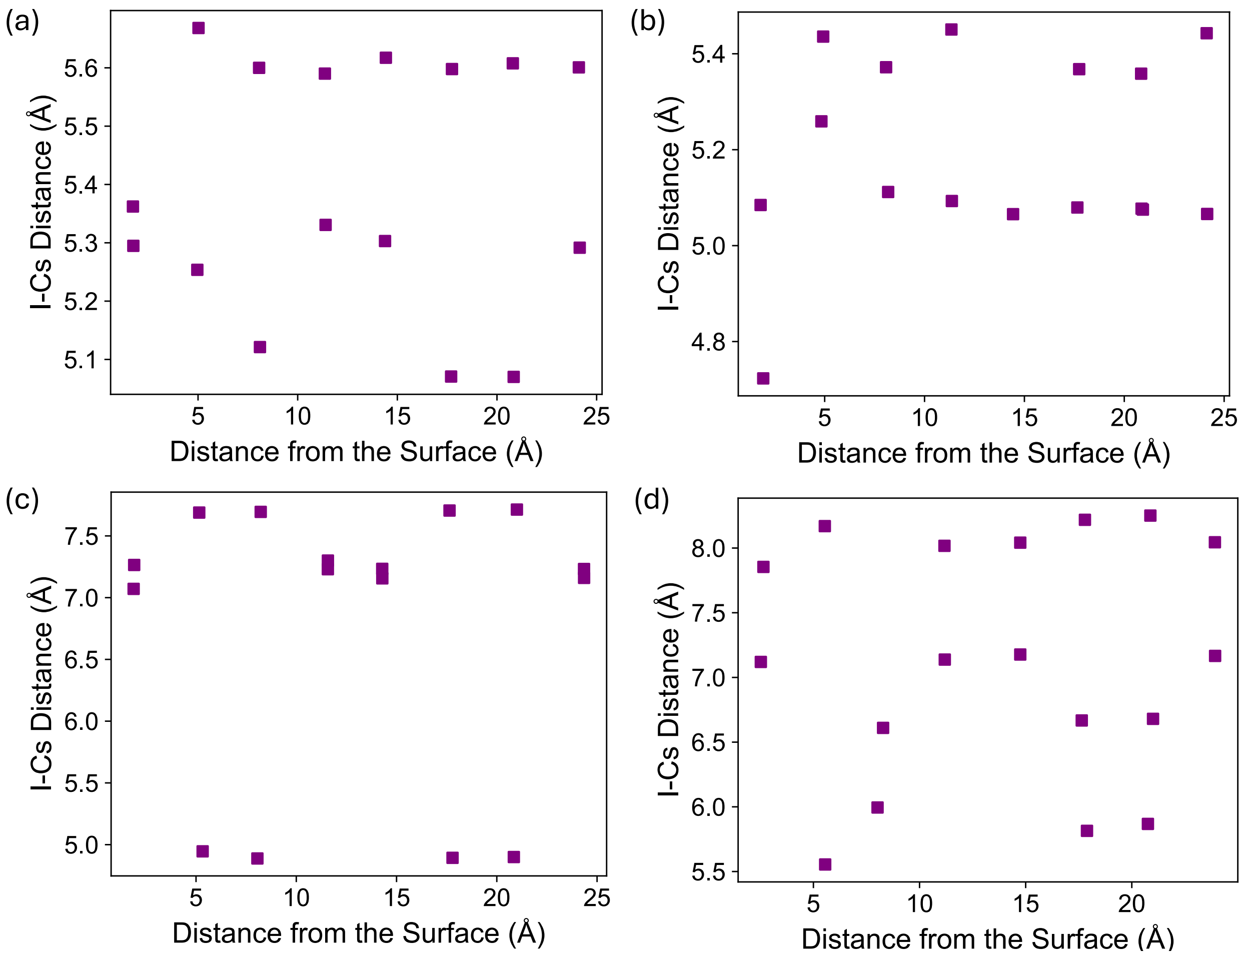


Figure S7: I-Cs distances plotted against the location of defects in $CsPbI_3$. It represents the variation of I-Cs distance for (a) $V_I^{\bullet}$, (b) $V_I^{\prime}$, (c) $I_i^{\bullet}$ and (d) $V_I^{\prime}$.

# References


(1) Larsen, A. H. et al. The atomic simulation environment—a Python library for working with atoms. *J. Phys.: Condens. Matter* **2017**, *29*, 273002.

(2) Momma, K.; Izumi, F. VESTA 3 for three-dimensional visualization of crystal, volumetric and morphology data. *J. Appl. Crystallogr.* **2011**, *44*, 1272–1276.
