# Supplementary material for: Modulation of Point Defect Properties Near Surfaces in Metal Halide Perovskites
Source: arXiv:2407.02249 source file (2024-07-02)

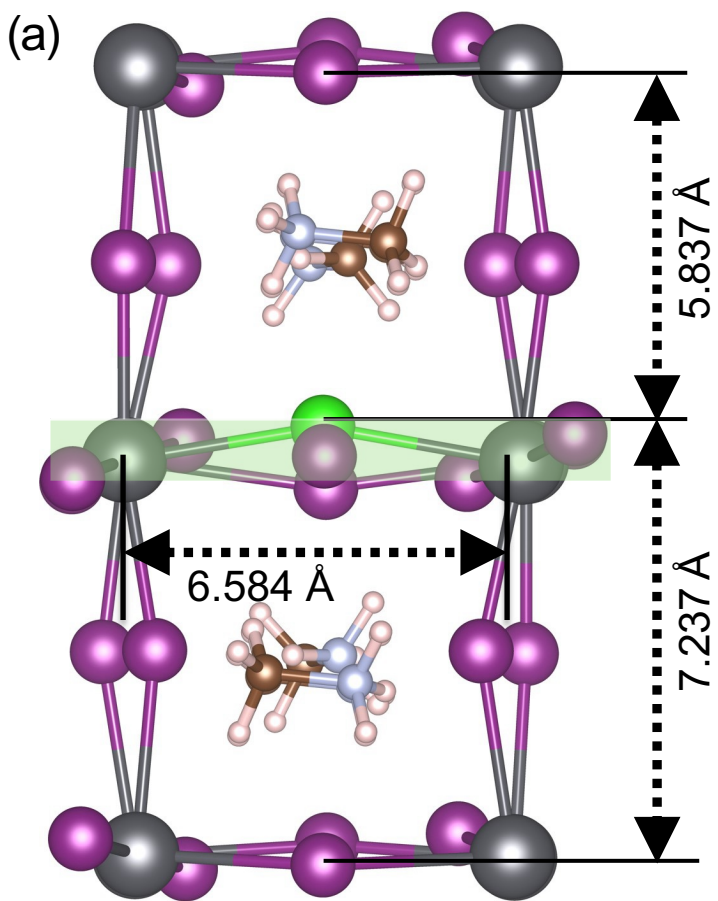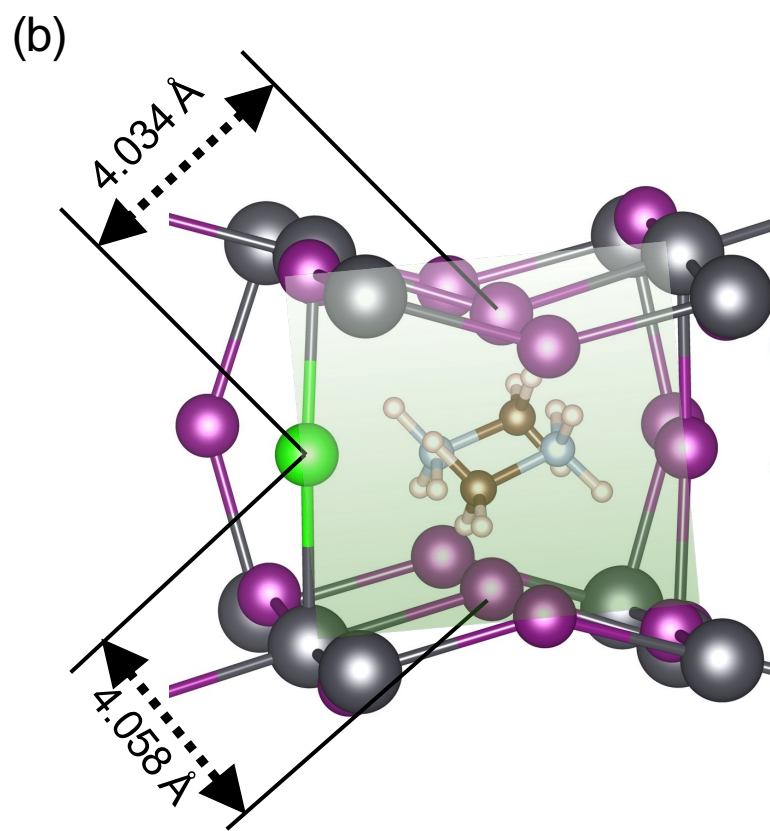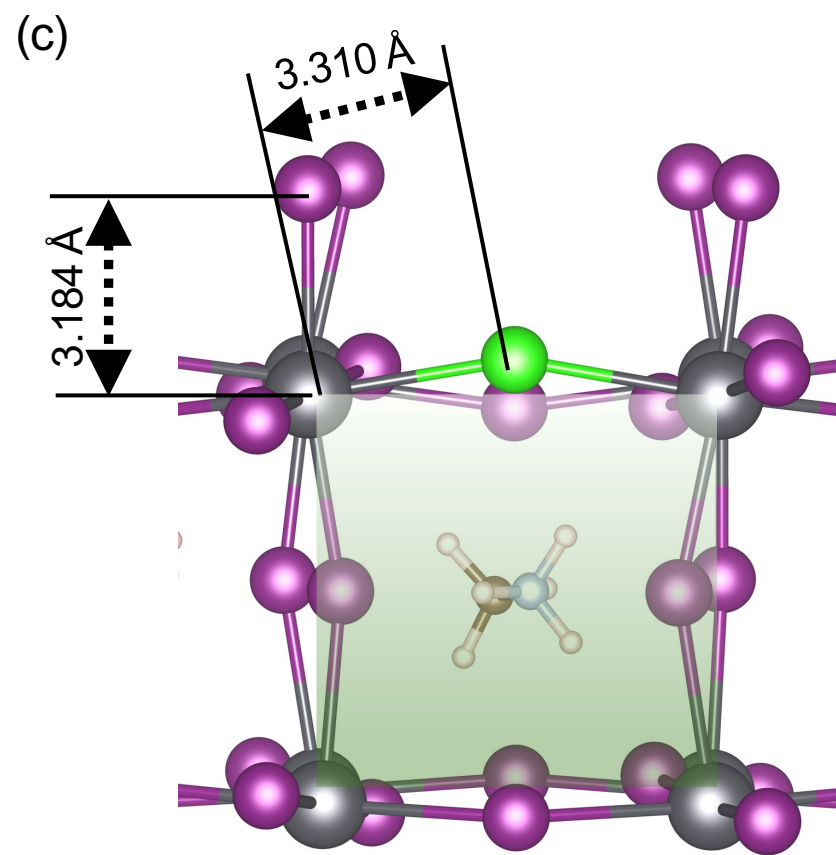

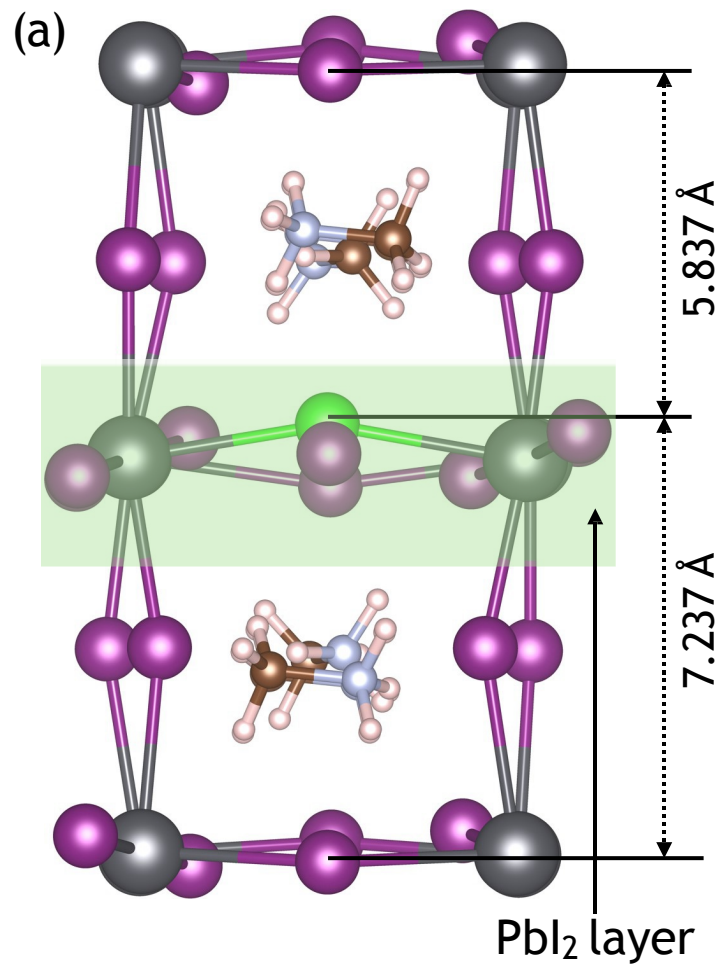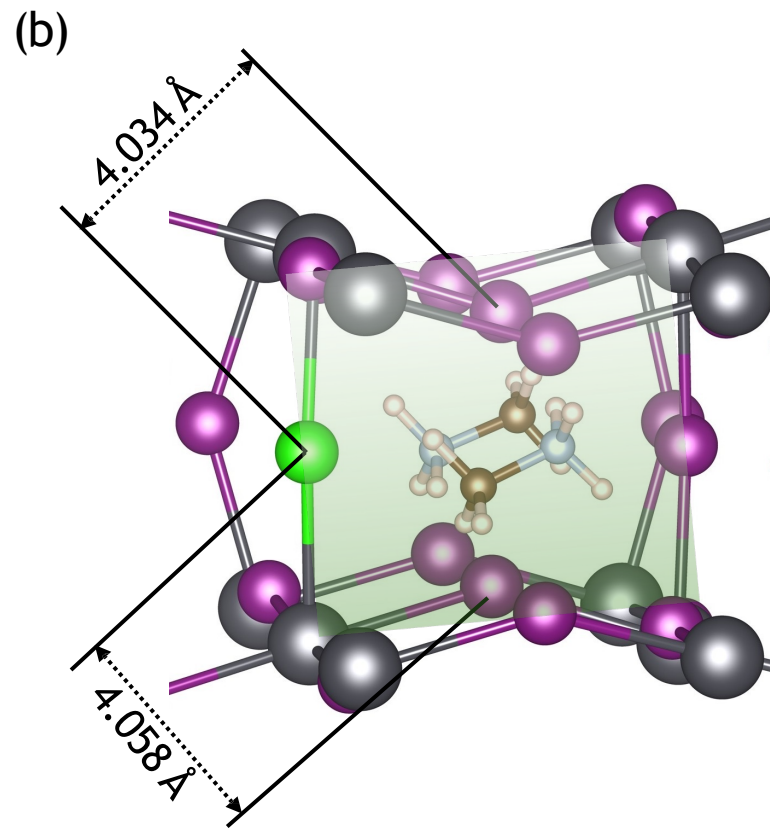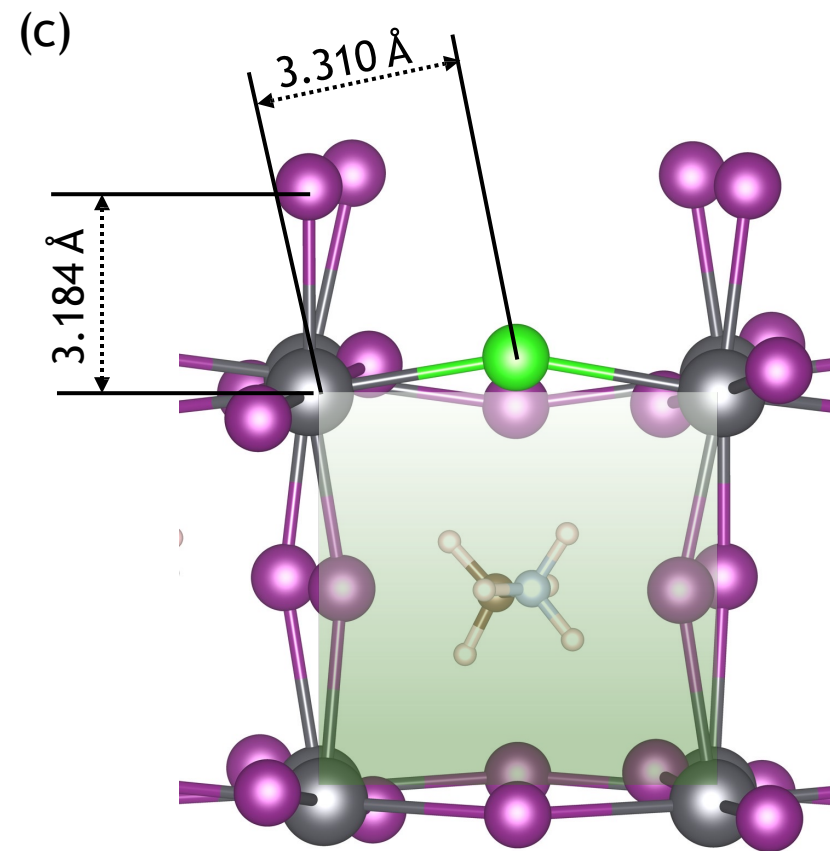

Supplement: Supplementary file 2 [file SI_1.pdf]
